# Supplementary material for: Band filling control of the Dzyaloshinskii-Moriya interaction in weakly ferromagnetic insulators
Source: arXiv:1704.00161 source file (2017-05-05)
Supplement: Supplementary file 1 [file supplemental.pdf]

# Band filling control of the Dzyaloshinskii-Moriya interaction in weakly ferromagnetic insulators
# (Supplemental Material)

G. Beutier,[1] S. P. Collins,[2] O. V. Dimitrova,[3] V. E. Dmitrienko,[4] M.I. Katsnelson,[5,6] Y.O. Kvashnin,[7] A.I. Lichtenstein,[6,8] V. V. Mazurenko,[6] G. Nisbet,[2] E. N. Ovchinnikova,[3] and D. Pincini[9,2]

[1]*Univ. Grenoble Alpes, CNRS, Grenoble INP, SIMaP, F-38000 Grenoble, France*
[2]*Diamond Light Source Ltd, Diamond House, Harwell Science and Innovation Campus, Didcot, Oxfordshire, OX11 0DE, UK*
[3]*M.V.Lomonosov Moscow State University, Leninskie Gory, Moscow 119991, Russia*
[4]*A. V. Shubnikov Institute of Crystallography RAS, Moscow 119333, Russia*
[5]*Radboud University Nijmegen, Institute for Molecules and Materials, Heyendaalseweg 135, NL-6525 AJ Nijmegen, The Netherlands*
[6]*Department of Theoretical Physics and Applied Mathematics, Ural Federal University, Mira str. 19, 620002 Ekaterinburg, Russia*
[7]*Department of Physics and Astronomy, Division of Materials Theory, Uppsala University, Box 516, SE-75120 Uppsala, Sweden*
[8]*I. Institut für Theoretische Physik, Universität Hamburg, Jungiusstraße 9, D-20355 Hamburg, Germany*
[9]*London Centre for Nanotechnology and Department of Physics and Astronomy, University College London, London WC1E 6BT, United Kingdom*

## SAMPLES

The quality of the samples is critical in the experimental part of this study. In particular, the chemical purity of the crystal plays an important role. The effect of doping with a different transition metal has been largely studied in $FeBO_3$ and $MnCO_3$. It has been shown that doping results in a sizable alteration of the magnetic properties, such as the spontaneous moment and the ordering temperature. In particular, doping $FeBO_3$ with Cr [1] and $MnCO_3$ with Fe [2, 3] has a huge and complex effect [4], because pure $CrBO_3$ and $FeCO_3$ are classical antiferromagnets with the moments parallel to the trigonal axis [5, 6]. The case of $MnCO_3$ is spectacular, since 0.5 % doping with Fe is sufficient to completely quench the weak magnetic moment [2, 3] and turn the resulting crystal into a classical antiferromagnet with the moments along the trigonal axis. It may explain the large dispersion of values found in the literature for $MnCO_3$. Doping with other elements also has a measureable effect, although not as spectacular, on the spontaneous magnetisation, the coercitive field and the Curie temperature [1]. There is to our knowledge no experimental study of the effect of doping in $CoCO_3$ and $NiCO_3$, but Moskvin predicted that mixing Mn and Ni in $Mn_{1-x}Ni_xCO_3$ would result in peculiar behaviors [7]. The results of Refs. [1], [2] and [3] suggest that the spontaneous magnetic moment and the Néel temperature of the samples are good indicators of the purity of the crystals. We present such measurements below.

### Sample growth

While $MnCO_3$, $CoCO_3$ and $FeBO_3$ macroscopic single crystals were available to us prior to this work, the project required a dedicated growth of $NiCO_3$ crystals, and macroscopic sizes were not achieved. The $NiCO_3$ crystals were synthesized at the Lomonosov Moscow State University, Faculty of Geology, by the hydrothermal method in standard autoclaves with a volume of 5-6 $cm^3$. Teflon was used as the protective coating. The coefficient of the autoclave filling was selected so that pressure was constant. The synthesis was carried out at the general pressure of 70-100 atm in the temperature range from 550 K to 560 K. The bottom temperature point was limited by kinetics of the chemical reaction while the upper point was limited by equipment characteristics. The experiment duration is 20 days and it corresponds to full completion of the chemical reaction. The following analytical-grade compounds were used: $NiCl_2$, $Na_2CO_3$, $B_2O_3$. The synthesis was carried out with the $NiCl_2$:$Na_2CO_3$:$B_2O_3$ ratio 1:1:1. Final cooling after synthesis to room temperature was done in 24 h. The precipitate was separated by filtering a stock solution, washed several times with hot distilled water and finally dried at room temperature for 12 h. Optical microscopy reveals that the precipitate is made of prismatic green crystals. Crystals were selected manually for further studies. Powder X-ray diffraction shows that white powder is a phase with the apatite-type structure. Element content of the selected single crystals was determined by inductively coupled plasma optical emission spectrometry and, independently, from the refinement of their crystal structure.

### Magnetic characterisation

Magnetization measurements were performed on single crystals from the same batches as those measured by X-ray diffraction by means of a SQUID vibrating-

TABLE I. Spontaneous magnetization at low temperature and critical temperature. Concerning the literature data of $MnCO_3$, only measurements performed on pure single crystals at low temperature ($T$<10 K) are reported, since it was reported that the magnetisation of powder samples is reduced [3] and that magnetic impurities also reduce the magnetisation [2, 3]. For $FeBO_3$ and $CoCO_3$ we provide two experimental values of the spontaneous magnetization (see text for details). The error bars of our experimental data is of the order of $10^{-5}$ $\mu_B$/ion. The critical temperature data selected from the literature concern the net magnetization; literature data measured on the antiferromagnetic part were discarded, although it is generally accepted that the onset of the weak ferromagnetic moment coincides with the onset of the antiferromagnetic order.

| | Spontaneous magnetization at low temperature ($\mu_B$/ion) | | Critical temperature (K) | |
|---|---|---|---|---|
| | Literature data | This work | Literature data | This work |
| $MnCO_3$ | 0.034 [8], 0.033 [3] | 0.035 | 32.43 [8] | 33.58±0.02 |
| $FeBO_3$ | 0.08 [9], 0.078 [10] | 0.071, 0.075 | 348.5 [9], 346.5 [10] | 345±0.5 [11] |
| $CoCO_3$ | 0.258 [12], 0.229 [13], 0.269 [14] | 0.255, 0.282 | 18.1 [12] | 17.76±0.02 |
| $NiCO_3$ | 0.372 [15], 0.412 [16], 0.391 [10] | - | 25.2 [15], 25.2 [16] | 23.83±0.06 |

sample magnetometer (VSM) at beamline I10 of the Diamond Light Source. The samples were glued on a quartz rod using GE Varnish. Magnetization vs field ($M\,vs\,H$) curves were measured at $T = 5$ K with the external magnetic field applied perpendicular to the $c$ axis of the trigonal structure, where the net magnetic moment of the canted antiferromagnetic structure resides, by sweeping the magnetic field in the sequence 0→ 5 kOe → -5 kOe → 0.

The $CoCO_3$ and $FeBO_3$ samples are in the form of relatively thin plates and the direction of the $c$ axis is easily identifiable as the orthogonal to the sample surface. In order to properly take into account the in-plane magneto-crystalline anisotropy, sets of measurements were repeated for: (i) two different orientations of the same crystal relative to the external magnetic field in the case of $CoCO_3$; (ii) two different crystals (with a generally different in-plane orientation) in the case of $FeBO_3$. The $c$ axis direction is not as obvious for the $MnCO_3$ sample. The magnetization in the latter was thus measured mounting the sample in three different orientations: the data set where $H \perp c$ can be assigned to the one displaying the strongest signal. The measurements corresponding to the other orientations were then discarded.

The magnetization curves show that, for values of the field large enough to completely orient the magnetic domains, the magnetic moment perpendicular to the $c$ axis, $m_\perp(H,T)$, exhibits the following linear dependence on the applied field $H_\perp$:

$$m_\perp(H,T) = m_0(T) + \chi_\perp(T)H_\perp \quad (1)$$

where $\chi_\perp(T)$ is the magnetic susceptibility in the $ab$ plane of the crystal and $m_0(T)$ is the spontaneous net magnetization (at zero field) arising from the moment canting. $m_0(T)$ can then be extracted extrapolating to zero field the $M\,vs\,H$ curves. Table I summarizes the results and compares them with data from the literature. $M\,vs\,H$ measurements were collected also for a single crystal of $NiCO_3$ that shows an analogous linear dependence of the magnetization as a function of the external field. However, due to the small size of the crystal, its mass could not be reliably determined and the magnetic moment per magnetic ion could not be calculated. For the other three samples, the spontaneous magnetization is similar to the values found in the literature.

Magnetization vs temperature measurements were also performed on $CoCO_3$, $MnCO_3$ and $NiCO_3$, in order to measure the critical temperature, corresponding to the onset of the weak ferromagnetic moment. The data were collected following the zero-field cooled (ZFC) - field-cooled (FC) protocol. The samples were first cooled below the Néel transition in zero field and the ZFC magnetization was then measured on warming by the application of a small field of 1 kOe for $CoCO_3$ and $MnCO_3$ and 5 kOe for $NiCO_3$. Once in the high temperature paramagnetic region, the FC magnetization was measured on cooling the samples down to 5 K keeping the field to the same value used for the ZFC data. The ZFC and FC data sets almost completely overlap, thus showing no significant irreversibility. The measured critical temperature also shows a good agreement with the literature data (Table I).

The temperature dependence of the magnetization was not measured for $FeBO_3$ because the SQUID apparatus does not allow to reach its critical temperature, which is above room temperature. Nevertheless, we reported the temperature dependence of a pure antiferromagnetic Bragg reflection in Ref. [11] and it also agrees well with literature data.

## X-RAY MAGNETIC AND RESONANT INTERFERENCE SCATTERING

### Magnetic structure in applied magnetic field

The magnetic structure of the crystals studied here is carried by the transition metal ions and consists of a stack along the $c$ axis of ferromagnetic layers at positions $z = n/6$ in hexagonal settings (Fig. 1). All the spins of a single layer are in plane and parallel to each other. Nearest-neighbour layers have antiferromagnetic

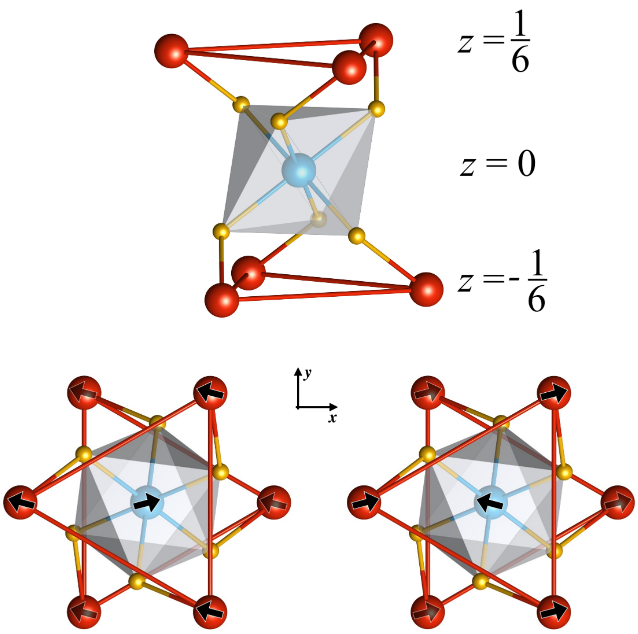


FIG. 1. Atomic and magnetic orders in weak ferromagnets $FeBO_3$, $MnCO_3$, $CoCO_3$ and $NiCO_3$. Boron and cabon atoms are omitted for clarity. The top panel indicates the local environment of a $3d$ atom and its six nearest-neighbor magnetic ions. The $z$ value denotes the coordinate along the $c$ axis of the hexagonal unit cell. Blue and red red spheres correspond to transition metal ions "1" and "2" in the text. The bottom left and right panels shows the two possible spin configurations, depending on the sign of the canting angle $\phi$, for a net ferromagnetic moment pointing to the bottom of the figure (left: $\phi < 0$; right: $\phi > 0$; see text for the definition of $\phi$).

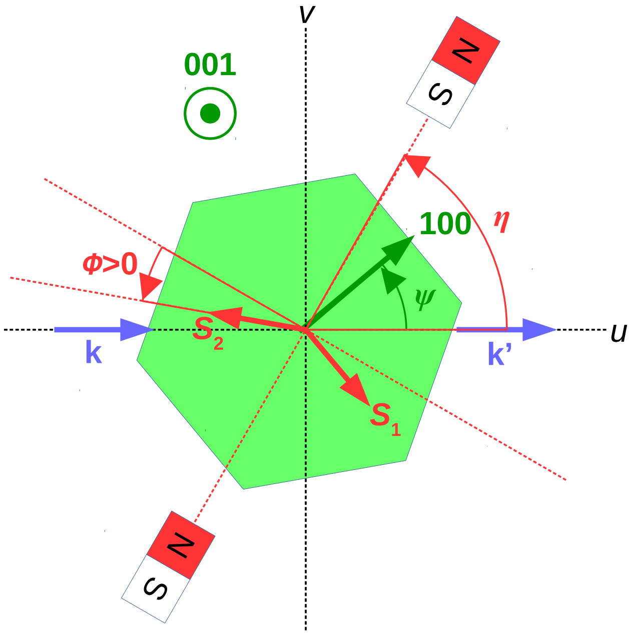


FIG. 2. A schematic view of the diffraction experiments. The orthogonal frame $(\hat{\boldsymbol{u}}, \hat{\boldsymbol{v}}, \hat{\boldsymbol{w}})$ is defined by $\hat{\boldsymbol{u}} = \frac{\boldsymbol{k}+\boldsymbol{k}'}{|\boldsymbol{k}+\boldsymbol{k}'|}$, $\hat{\boldsymbol{w}} = \frac{\boldsymbol{k}'-\boldsymbol{k}}{|\boldsymbol{k}'-\boldsymbol{k}|}$ and $\hat{\boldsymbol{v}} = \hat{\boldsymbol{w}} \times \hat{\boldsymbol{u}}$. The directions labelled "100" and "001" correspond to reciprocal space directions indexed in the hexagonal settings. The configuration shown here is the case $\phi > 0$. The directions of $\boldsymbol{S}_1$ and $\boldsymbol{S}_2$ are swapped when $\phi < 0$.

alignment, except for the twist induced by the DMI. We can thus describe the magnetic structure by considering only two spins $\boldsymbol{S}_1$ and $\boldsymbol{S}_2$ carried by the nearest-neighbor transition metal ions "1" and "2" at positions $(0, 0, 0)$ and $(1/3, 2/3, 1/6)$ respectively. To complete the definition of the system, it is necessary to be precise about the position of the oxygen atoms: they occupy the generic position $(x, 0, 1/4)$ of space group $R\bar{3}c$, with either $0 \leq x \leq 1/2$ or $1/2 \leq x \leq 1$. We use the first convention. The interaction between $\boldsymbol{S}_1$ and $\boldsymbol{S}_2$ is decribed by the exchange constant $J$ (considered isotropic for simplicity) and the Dzyaloshinskii vector $\boldsymbol{D}$ (the direction of $\boldsymbol{D}$ is reversed when the roles of $\boldsymbol{S}_1$ and $\boldsymbol{S}_2$ are swapped). The Hamiltonian in an external magnetic field $\boldsymbol{H}$ can be written:

$$\mathcal{H}' = J\boldsymbol{S}_1 \cdot \boldsymbol{S}_2 + \boldsymbol{D} \cdot [\boldsymbol{S}_1 \times \boldsymbol{S}_2] - \mu_B g \boldsymbol{H} \cdot [\boldsymbol{S}_1 + \boldsymbol{S}_2] \quad (2)$$

where $\mu_B$ is the Bohr magneton and $g \approx -2$ is the gyromagnetic ratio. In a weak external magnetic field ($\mu_B |g\boldsymbol{H}| \ll |\boldsymbol{D}|$) applied in the basal plane, the Hamiltonian minimizes the energy by rotating the net spin angular momentum $\boldsymbol{S}_{FM} = \boldsymbol{S}_1 + \boldsymbol{S}_2$ antiparallel to the applied field and by conserving the field-free magnetic structure with an antiferromagnetic spin structure factor $\boldsymbol{S}_{AFM} = \boldsymbol{S}_1 - \boldsymbol{S}_2$ in the basal plane and perpendicular to $\boldsymbol{S}_{FM}$. The sense of $\boldsymbol{S}_{AFM}$ is given by the sign of the component $D_z$ of $\boldsymbol{D}$ along the $c$ axis: when it is positive, the system minimizes its energy by canting $\boldsymbol{S}_1$ clockwise around the (001) axis and $\boldsymbol{S}_2$ anticlockwise (Fig. 1-2); the canting directions reverse with the sign of $D_z$. In the following, we note $\sigma_\phi$ the sign of $\phi$, which we define as equal as the sign of $D_z$. The situation is more complicated when considering the crystal field and the spin-orbit coupling. Nevertheless, the crystals of this study have easy magnetisation in plane with only weak anisotropy in the basal plane, such that this Hamiltonian describes the situation fairly well when the applied magnetic field is rotated in the basal plane and is strong enough to overcome the in-plane anisotropy. The latter decreases with temperature and can thus be reduced if necessary by approaching the Néel temperature [17].

In our experimental set-up (Fig. 2), the direction of the external magnetic field $\boldsymbol{H}$ in the laboratory frame is described by the angle $\eta$ rotating counterclockwise around the $c$ axis ($00L$ direction with $L > 0$) of the sample, with origin when $\boldsymbol{H}$ coincides in direction with $\boldsymbol{k} + \boldsymbol{k}'$. Following these considerations, the coordinates of $\boldsymbol{S}_{FM}$ and $\boldsymbol{S}_{AFM}$ in the orthonormal frame $(u, v, w)$ (Fig. 2) of the

laboratory are:

$$\boldsymbol{S}_{FM} = \boldsymbol{S}_1 + \boldsymbol{S}_2 = -2S\sin|\phi| \begin{pmatrix} \cos\eta \\ \sin\eta \\ 0 \end{pmatrix} \quad (3)$$

and

$$\boldsymbol{S}_{AFM} = \boldsymbol{S}_1 - \boldsymbol{S}_2 = 2S\sigma_\phi \cos\phi \begin{pmatrix} \sin\eta \\ -\cos\eta \\ 0 \end{pmatrix} \quad (4)$$

which is equivalent to the expression given in [11]:

$$\boldsymbol{S}_{AFM} = 2S\cos\phi \frac{\boldsymbol{H}\times\bar{\boldsymbol{D}}}{|\boldsymbol{H}|\,|\bar{\boldsymbol{D}}|} \quad (5)$$

where $\bar{\boldsymbol{D}}$ is the $\boldsymbol{D}$ vector averaged over the $M$-O-$M$ bonds of the crystals: it is by symmetry either parallel ($\sigma_\phi > 0$) or antiparallel ($\sigma_\phi < 0$) to the $c$ axis.

In $FeBO_3$ and $MnCO_3$, the orbital moment is quenched. In contrast, $CoCO_3$ and $NiCO_3$ have a strong orbital moment. Following the third Hund's rule, we assume that it is parallel (*not antiparallel*) to the spin. This assumption is confirmed by the *ab initio* calculations (see section "First-principles calculations" below). Equations (3) and (4) are hence also valid for the orbital moment (by replacing $S$ by $L$).

### Scattering model

According to Eq. (4), the sign of the DMI is encoded in the antiferromagnetic structure factor $\boldsymbol{S}_{AFM}$, hence in the magnetic scattering amplitude of neutrons or X-rays. Pure magnetic scattering reflections will however not provide the sign of the amplitude, and an interference between the magnetic scattering amplitude and a non-magnetic reference amplitude is needed. In order to interfere, both amplitudes must have same polarisation, not be out of phase, and have a similar magnitude. With neutrons, one can use the nuclear amplitude as the non-magnetic reference amplitude by measuring a reflection allowed by the space group symmetry of the nuclear structure which is not parallel to the trigonal axis [18]. The flipping ratio then provides the sign of the magnetic scattering amplitude. With X-rays, the same method would not work because the non-resonant non-magnetic (Thomson) scattering amplitude at space-group allowed reflections is several orders of magnitude larger than magnetic amplitudes, preventing from a reliable measurement of the interference. The Thomson amplitude can be used as reference amplitude at space-group forbidden reflections [19], where it vanishes in the kinematical theory of X-ray scattering but provides in fact a small residual amplitude due to dynamical multiple scattering effects. Here we used instead the X-ray diffraction method presented in Ref. [11]: we measure the interference between non-magnetic resonant scattering and magnetic non-resonant scattering at the $(0,0,6n+3)$ forbidden reflections. The resonant amplitude is of electric quadrupole origin, an exotic but well understood scattering process [20].

A reliable formalism for X-ray non-resonant magnetic scattering and X-ray resonant scattering is needed to exploit the interference signal. Since most X-ray resonant and/or magnetic scattering experiments care only about the intensity, many papers are not reliable as for the sign of the scattering factors and scattering amplitudes, or do not specify the adopted conventions. It is of course necessary to describe both scattering ampitudes with the same conventions of sign. However, a recent review paper by Grenier & Joly [21] deals explicitly with this problem. The formalism builds on that initially proposed by de Bergevin & Brunel for X-ray non-resonant magnetic scattering [22] and used in Ref. [11]. Based on this formalism, we derive below the relation between the intensity measurement and the sign of the DMI.

In this formalism, the X-ray non-resonant magnetic scattering factor $f_{mag}$ of the antiferromagnetic spin structure is purely imaginary. Following [22] and [21], it can be written, in the case of incident polarisation $\sigma$ (perpendicular to the scattering plane) and scattered polarisation $\pi$ (in the scattering plane) [1] :

$$f_{mag}^{\sigma\pi} = -i\frac{\hbar\omega}{mc^2}\sin^2\theta\left[\boldsymbol{L}(\boldsymbol{q})\cdot(\hat{\boldsymbol{k}}+\hat{\boldsymbol{k}'}) + 2\boldsymbol{S}(\boldsymbol{q})\cdot\hat{\boldsymbol{k}}\right] \quad (6)$$

where $\hbar\omega$ is the X-ray energy, $mc^2$=511 keV is the rest mass of the electron, $\theta$ is the Bragg angle, and $\boldsymbol{L}(\boldsymbol{q})$ and $\boldsymbol{S}(\boldsymbol{q})$ are the orbital and spin structure factors at the reciprocal lattice vector $\boldsymbol{q} = \boldsymbol{k'} - \boldsymbol{k}$. In the case of the $(0,0,6n+3)$ forbbiden reflections:

$$\boldsymbol{L}(\boldsymbol{q}) = \boldsymbol{L}_{AFM} f_L(\boldsymbol{q}) \quad (7)$$

$$\boldsymbol{S}(\boldsymbol{q}) = \boldsymbol{S}_{AFM} f_S(\boldsymbol{q}) \quad (8)$$

where $f_L(\boldsymbol{q})$ and $f_S(\boldsymbol{q})$ are respectively the orbital and spin form factors. By considering Eq. (4), Eq. (6) becomes:

$$f_{mag}^{\sigma\pi} = -i\sigma_\phi f_m \sin\eta \quad (9)$$

where $f_m$ is a real positive quantity:

$$f_m = 2\frac{\hbar\omega}{mc^2}\left[Lf_L(\boldsymbol{q}) + Sf_S(\boldsymbol{q})\right]\cos\phi\sin 2\theta\sin\theta \quad (10)$$

The charge scattering factor consists of two parts: non-resonant Thomson scattering and resonant scattering $f_{res}$. The former cancels out at reflections $(0,0,6n+3)$

[1] the scattering amplitude is $-r_e f_{mag}$ with $r_e = e^2/mc^2$ the classical electron radius. Here we work with the scattering factors for both the charge and magnetic terms.

owing to the space-group symmetry, but the latter does not. Resonant scattering is normally written as a series of electric multipolar resonances [20, 21]. The largely dominant term is the electric dipole-dipole (E1E1) unless it cancels out by symmetry, which is the case here at the (0,0,$6n+3$) reflections due to the high symmetry of the sites hosting the resonant atoms. The two next most-common terms are the electric dipole-quadrupole (E1E2), which cancels out similarly to the E1E1 term, and electric quadrupole-quadrupole (E2E2). Higher order electric multipoles and multipoles involving magnetic transitions are exotic and much weaker. We are thus left with a single term, E2E2, for which the formalism [20, 21] provides a simple expression:

$$f_{res}^{\sigma\pi} = Q\left(E\right)\cos 3\psi \tag{11}$$

where $Q(E) = Q'(E) + iQ''(E)$ is a complex spectrum [2] and $\psi$ is the azimuthal angle of the reflection (Fig. 2). Here, $\psi = 0$ when the 100 reciprocal direction is parallel (*not antiparallel*) to $\hat{\boldsymbol{k}} + \hat{\boldsymbol{k}}'$. Importantly, with incident polarisation $\sigma$, $f_{res}$ is null in the unrotated polarisation channel. The interference between magnetic scattering and resonant scattering can therefore only be measured in the rotated channel. It is also remarkable that a single time-even spectroscopic term contributes to the forbidden reflection, since the general E2E2 tensor can have up to 15 independent tensor components in absence of symmetry [23].

In principle, there is also X-ray resonant magnetic scattering (XRMS). Its electric dipole resonance is usually the strongest, although the magnetic shell is probed only inderectly at the K edge of 3d transition metals. Following Hill and MacMorrow [24] and using the same expressions as above, we can write its contribution as:

$$f_{XRMS}^{\sigma\pi} = 2iF^{(1)}(E)\sigma_\phi \cos\phi\cos\theta\sin\eta \tag{12}$$

It has thus the same $\sin\eta$ dependence as non-resonant magnetic scattering. In contrast, it is not spectroscopically flat, due to the spectroscopic term $F^{(1)}(E)$. Owing to its electric dipole origin, it is expected to be spectroscopically separated from the E2E2 resonant term, hence not providing useful interference for the determination of the DMI sign. Moreover, extracting $\sigma_\phi$ from this term would require reliable calculations of $F^{(1)}(E)$, which is complex. The same remark also holds for a possible resonant magnetic scattering from the electric quadrupole. The latter has a more complicated angular dependence, involving $\sin(n\eta)$ terms with $n$ =1, 2, 3 [24]. It is expected to peak roughly at the same energy as the resonant non-magnetic scattering. Exploiting the non-resonant magnetic scattering is therefore simpler, if one can discard the resonant magnetic scattering. We do so because of the spectroscopic separation (dipole contribution) or its presumed weakness (quadrupole contribution): the occurrence of significant Fourier harmonics of order larger than 2 (in particular $\sin 3\eta$ or $\sin^2(3\eta)$ terms) in the $\eta$ dependence of the intensity would invalid this assumption.

When considering only the non-resonant magnetic scattering and the resonant non-magnetic scattering, the total intensity measured with a polarisation analyser in the channel $\sigma \to \pi$ is:

$$I^{\sigma\pi} = \left|f_{mag}^{\sigma\pi} + f_{res}^{\sigma\pi}\right|^2 = I_{mag} + I_{res} + I_{interf} \tag{13}$$

which is composed of the pure magnetic term $I_{mag}$, the pure resonant term $I_{res}$, and the interference term $I_{interf}$:

$$I_{mag} = f_m^2 \sin^2\eta \tag{14}$$

$$I_{res} = |Q(E)|^2\cos^2 3\psi \tag{15}$$

$$I_{interf} = 2\sigma_\phi f_m Q''(E)\cos 3\psi\sin\eta \tag{16}$$

The determination of the sign $\sigma_\phi$ relies thus on the knowledge of the resonant spectrum $Q''(E)$. The latter is calculated with the software FDMNES, which is based on the formalism given in [21]. [3]

We have already shown that this model is reliable in the case of $FeBO_3$, and in particular that the magnetic scattering and resonant scattering measured independently (off-resonance and above the Néel temperature respectively) behave as expected [11]. Moreover, Eq. (16) shows that there are three ways to reverse the interference effect: with the magnet angle $\eta$, with the azimuthal angle $\psi$, and possibly with the X-ray energy $E$ if $Q''(E)$ takes positive and negative values (Fig. 3), as seen in $FeBO_3$ [11].

## Experimental method

The X-ray diffraction measurements were performed on single crystals of millimiter size, except for $NiCO_3$ which was a grain of less than 100 $\mu$m, hence the lower quality of the data for this material. The experiments were performed at beamline I16 of Diamond Light Source with preliminary measurements at beamline XMaS of the European Synchrotron Radiation Facility. The 009 forbidden reflection of the four crystals was measured in vertical Bragg geometry using the natural linear horizontal

[2] $Q(E)$ is a unique spectrum for all forbidden reflections of the type $(0,0,6n+3)$ of a given crystal of the series studies here, except that it scales with $\cos^3\theta$.

[3] The output of FDMNES is given in the X-ray crystallographic convention, which reverses the direction of time compared to the standard physical convention used in [22] and [21]. As a consequence, the complex conjugate of the FDMNES output is taken to be consistent with the formalism used here.

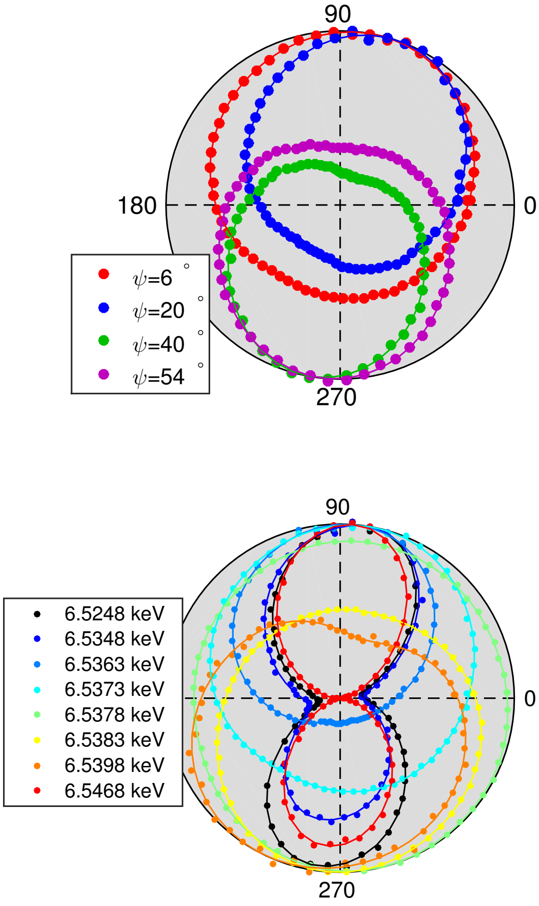


FIG. 3. Selected magnet scans of $MnCO_3$ (solid circles) with their trigonometric fits (lines). All curves are normalized to their maximum value. Top: at $E = 6.5373$ keV for various values of the azimuth $\psi$. The sign of the interference changes with $\cos 3\psi$ (Eq. (16)). Bottom: at $\psi = 6°$ for various values of the energy. Far from the resonance (6.5248 keV), the intensity is symmetric. At the peak of the quadrupolar resonance (6.5378 keV), the intensity is nearly independent of the magnet direction. The interference changes sign across the resonant peak, revealing a change of sign of the resonant amplitude. The intensity at 6.5468 keV is dominated by XRMS and is nearly symmetrical. These selected energies are highlighted in Fig. 4.

($\sigma$) polarisation of the source and a polarisation analyser to selected the rotated polarisation ($\pi$) of the scattered beam. The reflections used for the polarisation analysis were: the 220 refflection of copper ($FeBO_3$ and $MnCO_3$), the 006 reflection of graphite ($CoCO_3$) and the 222 reflection of copper ($NiCO_3$). The measurements were performed around the K edge of the transition metal, with the quadrupolar resonance found at $\sim$ 6.538 keV ($MnCO_3$), $\sim$ 7.112 keV ($FeBO_3$), $\sim$ 7.708 keV ($CoCO_3$), and $\sim$ 8.332 keV ($NiCO_3$) for the data taken at I16. The crystals were mounted in a close-cycle cryostat (except for $FeBO_3$) and the measurements were performed below the Néel temperature: at 300 K ($FeBO_3$), 7 K ($MnCO_3$), 13 K ($CoCO_3$) and 5.5 K ($NiCO_3$). In the case of $CoCO_3$, the temperature was chosen in order to obtain a sufficiently small in-plane magneto-crystalline anisotropy (which is easily evidenced on the data set when it is strong [17]). The other samples were found to have negligible in-plane anisotropy. Two permanent magnets mounted on a rotation stage and surrounding the crystal were used to apply magnetic field ($\sim$ 0.01 T) in its basal plane.

The data sets consist of the following measurements: for sereral azimuthal angles $\psi$ carefully chosen to avoid Renninger reflections, the energy of the incident X-rays was varied across the resonance. For each energy, the 009 reflection was first carefully aligned, and a 360° $\eta$-scan was recorded with all other motors fixed. As already reported, this method allows to obtain very high quality data, since the sample does not move with respect to the beam during the $\eta$-scan [11, 25].

## Experimental results

Following Eq. (13)–(16), each $\eta$-scan was fitted as a series of trigonometric terms in $\eta$. However, while these equations suggest that a constant, a $\sin\eta$ and a $\sin^2\eta$ terms should be sufficient, we found necessary to add a $\cos\eta$ term. This term accounts for a loss of symmetry between the two directions of the magnet in the scattering plane, *i.e.* parallel and antiparallel to $\boldsymbol{k} + \boldsymbol{k'}$, while the model predicts an asymmetry only in the two directions transverse to the scattering plane. The results of the fits are presented in Fig. 4.

The pure resonant spectrum $|Q(E)|^2$ is given by the constant term (Eq. (15)). In all crystals except $MnCO_3$, it shows a single resonance and vanishes away from the resonance. In $MnCO_3$, there is a secondary resonance about 4 eV above the main one. While the main resonance has the expected azimuthal dependence in $\cos^2 3\psi$ (Eq. (11)), the secondary one does not. Its origin is not clear, but it is not involved in the interference term we are interested in. The other three crystals have a single resonance, but the normalization by $\cos^2 3\psi$ is not as good as for the main resonance of $MnCO_3$. The discrepency can be due to the inhomogeneity of the samples combined with the sphere of confusion of the diffractometer. One curve of $FeBO_3$ and one curve of $NiCO_3$ have significant tails. It suggests the occurrence of a weak multiple diffraction amplitude for these particular azimuths. This is a common effect when measuring forbidden reflections, even though great care was taken in the choice of the azimuthal values to minimize it.

The pure magnetic intensity (Eq. (14)) is given by the $\sin^2\eta$ term. When considering only the non-resonant magnetic scattering, it should be spectroscopically flat,

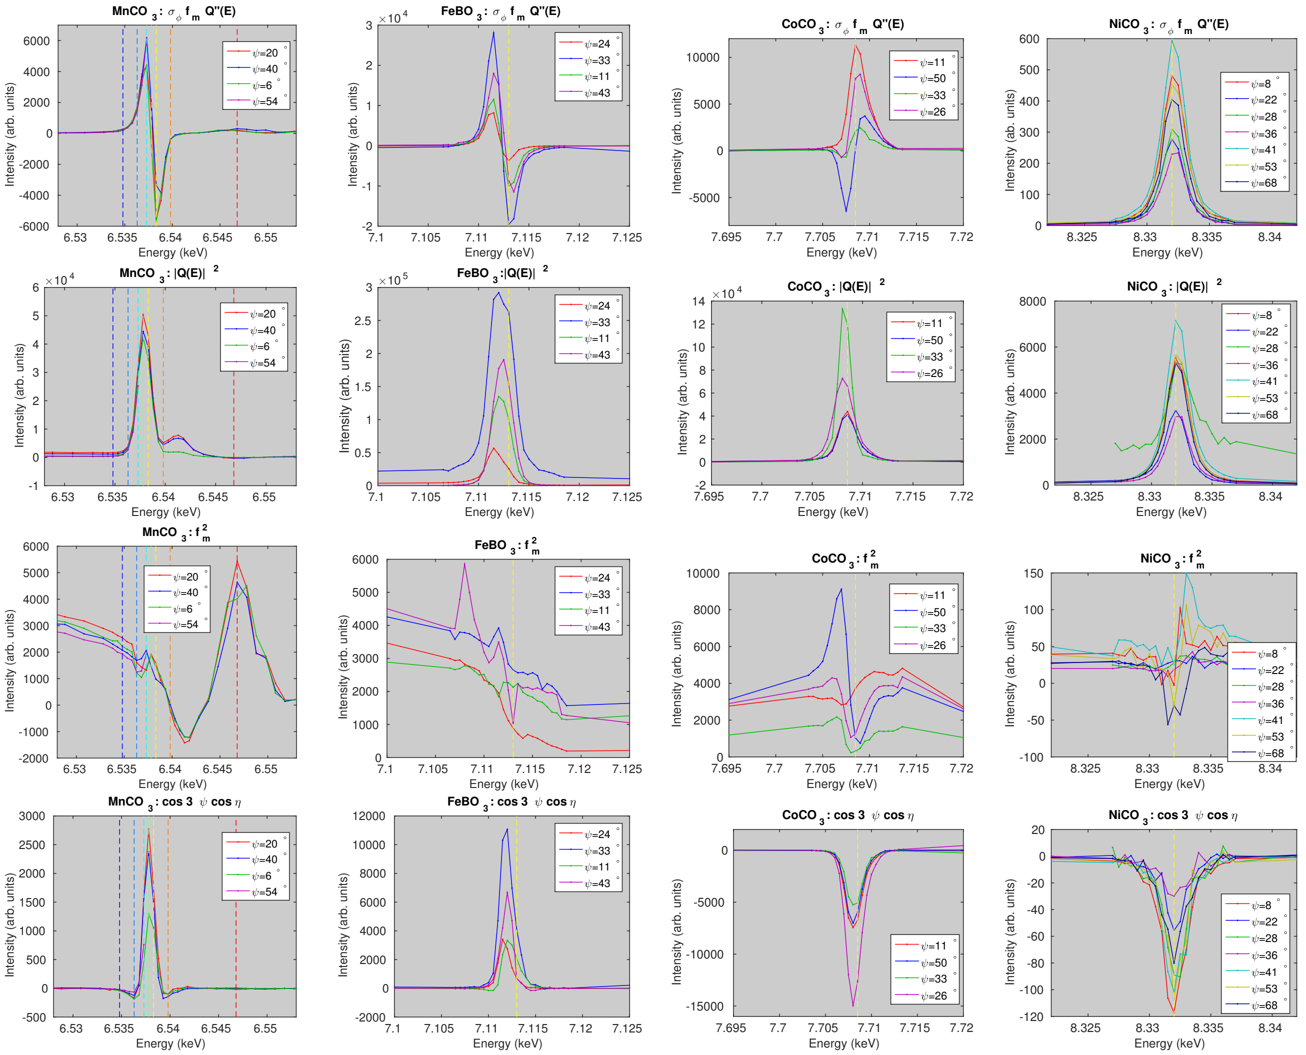


FIG. 4. Spectra obtained by fitting the $\eta$-scans with trigonometric functions, at several azimuths. From top to bottom: interference term $\sigma_\phi f_m Q''(E)$, proportional to $\sin\eta$ and normalized by $\cos 3\psi$; pure resonant term $|Q(E)|^2$ constant in $\eta$ and normalized by $\cos^2 3\psi$; pure magnetic term $f_m^2$ proportional to $\sin^2\eta$ and constant in $\psi$; additional term of unknown origin, proportional to $\cos\eta$ (arbitrarily normalized by $\cos 3\psi$). The vertical dash lines mark the energies shown in Fig. 3 in the case of $MnCO_3$. The yellow vertical dash lines mark the energies shown in Fig. 2 of the letter for all crystals.

except for the self-absorption effect (the self-absorption effect is not corrected in the data presented here): the case of $FeBO_3$ corresponds well to this case. However in $MnCO_3$ we observe a peak around 6.547 keV. It is most probably due to resonant magnetic scattering, which has the same $\eta$ dependence as the non-resonant magnetic scattering (Eq. 12) and occurs at higher energy than the quadrupolar resonance, owing to its electric-dipole nature. Resonant magnetic scattering is also observed in $CoCO_3$, but weaker and broader in energy. The case of $NiCO_3$ is not clear because of the lower quality of the data. We also note a clear negative magnetic intensity in $MnCO_3$ at the same energy as the secondary resonant term seen on $|Q(E)|^2$. This negative intensity does not make sense and confirms an unexplained contribution in this energy range. It is nevertheless away from the interference region and does not compromize the analysis of the DMI sign.

The interference term (Eq. (16)) is given by the $\sin\eta$ term. It provides a determination of $\sigma_\phi Q''(E)$, where $\sigma_\phi$ is independent of the energy. As expected, it is a resonant term and vanishes away from the resonance. After normalization by $\cos 3\psi$, this term should be independent of the azimuth $\psi$. The normalization works well for $MnCO_3$. In the case of $FeBO_3$ and $NiCO_3$, the various curves are similar to each other, except for a positive scaling factor. The case of $CoCO_3$ is more surprizing, because the curves obtained at various azimuths are not completely similar to each other. Nevertheless, as far as we are concerned only with the sign of the DMI, we can rely on the upper side of the spectrum, which keeps the same sign at all measured azimuths. In any case, we can

thus compare these spectra with the FDMNES calculation of $Q''(E)$ and, if they match (for either value of $\sigma_\phi$), we conclude that the FDMNES spectrum is reliable, *including its sign.* Then the sign $\sigma_\phi$ comes straightforward. This is discussed in the next section.

The magnitude of the additional $\cos\eta$ term is found smaller but comparable to the expected interference term, in particular in the case of $CoCO_3$. Its spectrum shows a clear resonance at the same position as the $\sin\eta$ term. It is interesting to note that the amplitude of the resonance is positive for $MnCO_3$ and $FeBO_3$ and negative for $CoCO_3$ and $NiCO_3$, hence matching the conclusions on the sign of the DMI. Moreover, based on only a few azimuthal values, it seems to have the same $\cos 3\psi$ dependence. These three features point at the same origin as the known interference term. A possible cause of this unexpected term arises from the intrinsic limitations of the 'standard' models of anisotropic resonant x-ray scattering. In the absence of magnetism, a symmetry-based approach picks out the resonant scattering tensor components that are consistent with crystal electric field at the atomic sites. Quantitative values of the tensor components can be computed via electronic structure codes, such as FDMNES. Such a model is essentially exact. However, for 'magnetic' resonant scattering, including magnetically-driven time-even anisotropy, one typically adopts a simplified model [24] whereby crystal field effects and crystal symmetry are ignored, and cylindrical symmetry about the magnetic moments is assumed. A more complete picture should include both crystal field and magnetic interactions in a uniform framework. Such a framework is beyond the scope of the present report.

## FDMNES calculations

The FDMNES software [26] was used to calculate the resonant scattering factor $f^{\sigma\pi}_{res}$. The calculations were performed using the structural parameters available in the literature [27–29], ignoring the magnetic structure, and using the finite difference method [30] with standard parameters. A crucial point is to describe the structure in a way that is consistant with the definition of the antiferromagnetic structure factor $\boldsymbol{S}_{AFM}$: when describing the crystals in the hexagonal settings of the $R\bar{3}c$ space group, the oxygen atoms are located at $(x,0,1/4)$ in reduced lattice units with $0 \leq x \leq 1/2$ (the opposite decription is $1/2 \leq x \leq 1$). Switching choices simply reverses the sign of the resonant amplitude.

The most important parameter of the calculations to tune the resonant amplitude is the value of the Fermi energy, which determines the cut-off in the convolution of the empty states used for the electronic transition. The resonant scattering factor resembles a double-Lorentzian [11], whose lower resonance can be truncated, depending on the choice of the Fermi level (Fig. 5):

$$Q(E) = \frac{A_1}{(E - E_0 + \Delta/2) - i\Gamma} + \frac{A_2}{(E - E_0 - \Delta/2) - i\Gamma} \tag{17}$$

where $A_1 \leq 0$ and $A_2 > 0$ are the amplitudes of the Lorentzian resonances, $E_0$ the mean resonance energy, $\Delta$ their separation in energy, and $\Gamma$ their common width. We did not find a reliable way to predict the Fermi energy, and its value was therefore tuned to obtain the best fit to the spectrum determined by X-ray diffraction (with either sign). The values of $\alpha = |A_1/A_2|$ resulting from the fits are plotted in Fig. 5.

The resonant spectra $Q''(E)$ are shown in Fig. 6. We found that, in the case of $FeBO_3$ and $MnCO_3$, the double-Lorentzian is not truncated, while in the case of $NiCO_3$ the first Lorentzian is fully truncated. Moreover the measurements obtained at different azimuths $\psi$ are consistent. The case of $CoCO_3$ is intermediate and problematic: the first Lorentzian is partially truncated with a cut-off value that is different depending on the azimuthal values. Let us recall that $CoCO_3$ is also the crystal for which we find the largest unexplained $\cos\eta$ term. These two issues point at the limits of the model in this case, and again suggest that the symmetry may be lowered by the magnetic field, hence enabling different resonant terms. We note that the case of $NiCO_3$ is not problematic, although it has a larger orbital moment than $CoCO_3$, so that the presence of a strong orbital moment, which is quenched in $FeBO_3$ and $MnCO_3$, is not the origin of the problem. Despite the difficulty to define a unique Fermi level for $CoCO_3$, there is a tendency over the four crystals to increase the Fermi level with the filling of the $3d$ shell.

Importantly, since the calculated spectra have the same shapes before convolution of the empty states and the convolution truncates only the first Lorentzian, the second part of the convoluted spectrum is common to all four crystals. It is therefore reliable to compare the signs of the DMI based on measurements performed in the upper part of resonance, as presented in Fig. 3 of the Letter (care was taken to also chose azimuths all in the range $0 < \psi < 30°$, in which $\cos 3\psi > 0$).

## Temperature dependence of the DMI sign in CoCO3

Petrov *et al.* observed in $FeBO_3$ that the magnitude of the canting angle does not change with temperature once the magnetic order is established [9]. A similar observation has been made in the orthoferrites $RFeO_3$, another group of weak ferromagnets [31]. Both studies point out that this behavior is expected from the molecular field theory of the DMI. Nevertheless, these experimental studies deal only with the magnitude of the canting angle and there is so far no experimental confirmation

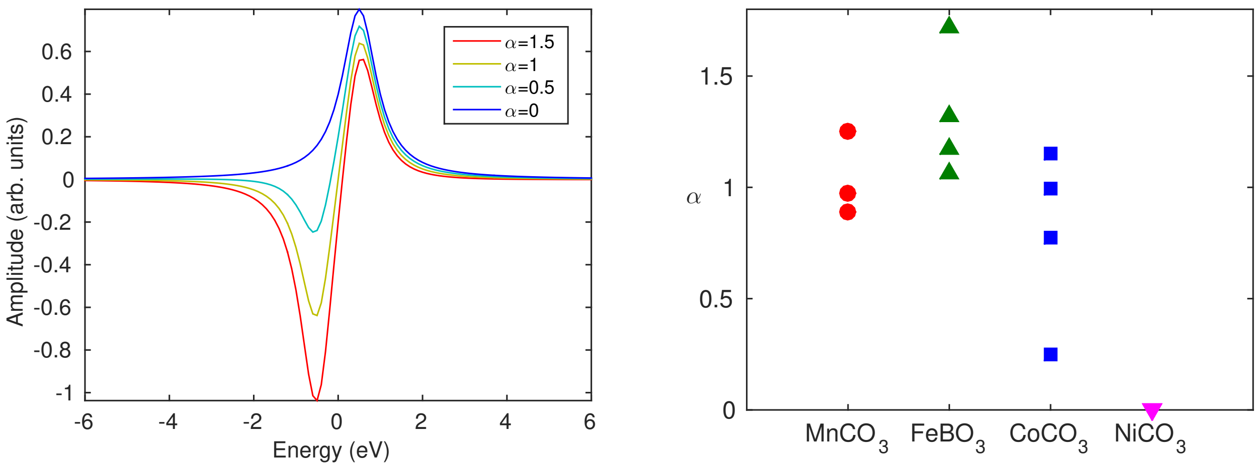


FIG. 5. Resonant spectra $Q''(E)$. Left: double-Lorentzian model, for various values of the parameter $\alpha = |A_1/A_2|$ (the ratio between the positive and negative Lorentzian amplitudes). The curves are arbitrarily centred at $E_0 = 0$, the parameters $\Delta$ and $\Gamma$ are set to 1 eV, and $A_2$ to 1 (arb. units). $FeBO_3$ corresponds roughly to the case $\alpha = 1.5$; $MnCO_3$ corresponds roughly to the case $\alpha = 1$; $CoCO_3$ corresponds roughly to the cases $\alpha = 1.5$, 1 and 0.5, depending on the azimuth; $NiCO_3$ corresponds well to the case $\alpha = 0$. Importantly, in the four cases, the amplitude is positive in the right part of the spectrum. Right: experimental values found for $\alpha$ at the azimuths given in Fig. 6.

that its sign does not reverse with temperature.

We measured the temperature dependence of the 009 reflection of $CoCO_3$ at energy and azimuth for which the interference term is strong (Fig. 7). The resonant amplitude is not expected to change with temperature since the crystal structure changes little in this temperature range. The data were recorded without the polarisation analyser: in the $\sigma \to \sigma$ channel, which adds incoherently to the $\sigma \to \pi$ one, the resonant amplitude is zero, and the non-resonant magnetic scattering amplitude varies like $\cos\eta$, such that the intensity contribution of the $\sigma \to \sigma$ channel varies like $\cos^2\eta$ and mixes with the constant and $\sin^2\eta$ terms of the $\sigma \to \pi$ intensity. The temperature dependence of the $\sin\eta$, $\cos\eta$ and $\sin^2\eta$ terms are shown in Fig. 7. The $\sin\eta$ and $\cos\eta$ describe a typical magnetization curve, with a Néel temperature at 17 K, close to the literature data (18 K) [12]. Interestingly, both terms follow the same temperature dependence, which suggest that the unknown term in $\cos\eta$ is also linear with the magnetisation (or more precisely with the antiferromagnetic order). Concerning the sign of the DMI, since the $\sin\eta$ term is proportional to $\sigma_\phi\,[S(\boldsymbol{q}) + L(\boldsymbol{q})]$ via a temperature-independent prefactor (Eq. (10) and (16)), it is clear that it does not change once the magnetic order is established. According to standard formula of pure non-resonant magnetic scattering taking into account both polarisation channels [32], the $\sin^2\eta$ term is expected to be a linear function of $S^2(\boldsymbol{q})$ and $(S(\boldsymbol{q}) + L(\boldsymbol{q}))^2$ and therefore it varies like the square of the $\sin\eta$ term, assuming that $S(\boldsymbol{q})$ and $L(\boldsymbol{q})$ have the same temperature dependence. Figure 7 supports this assumption.

## FIRST-PRINCIPLES CALCULATIONS

### Computational details

To simulate the electronic structure and magnetic properties of carbonates we used the Vienna *ab initio* simulation package [33] (VASP) within local density approximation taking into account the on-site Coulomb interaction and spin-orbit coupling [34] (LSDA+$U$+SO). The projector augmented-wave [35, 36] pseudopotentials have been employed. In these calculations the maximal energy of the plane waves was set to 650 eV. The energy convergence criterium of $10^{-7}$ eV and the $k$-point grid with up to 8×8×8 divisions over the full Brillouin zone were used. The static Coulomb correlations between the $3d$ electron on the transition metal ions were added within a simplified rotationally-invariant scheme proposed by Dudarev [37]. For each system the value of the on-site Coulomb interaction ($U$=3 eV for $MnCO_3$, $U$ = 4 eV for $FeBO_3$, $U$ = 3 eV for $CoCO_3$ and $U$=4 eV for $NiCO_3$) was chosen to obtain the best agreement on the absolute values of the canting angles with experimental data taken from the literature. The Hund's $J$ was assumed to be system-independent and set to 0.9 eV for all the systems. All studied compounds were considered in their experimental crystal structures, found in Refs. [27–29].

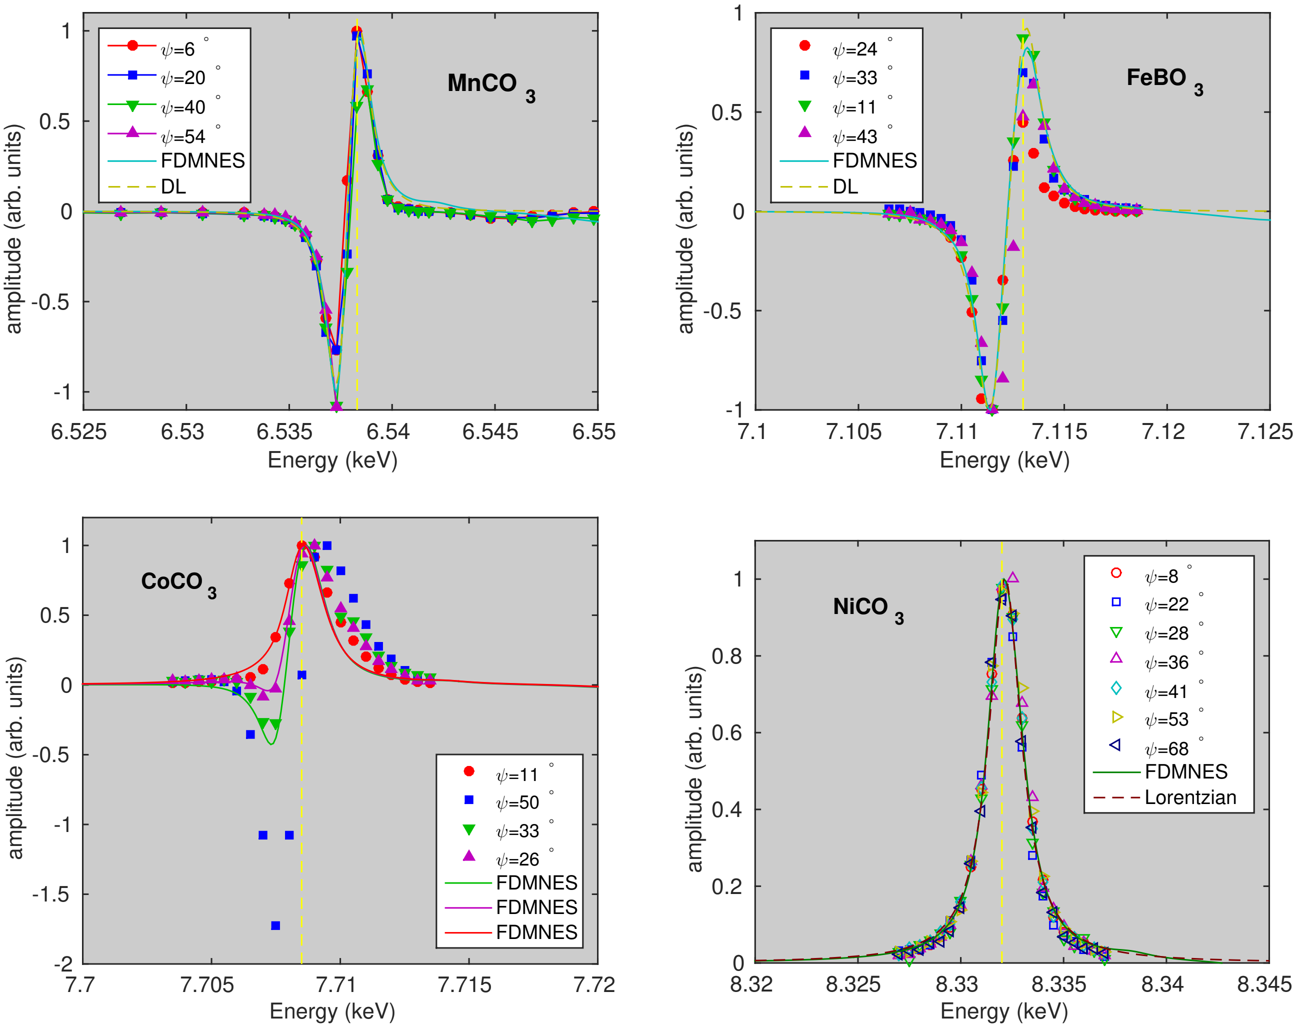


FIG. 6. Resonant spectra $Q''(E)$ (normalized to the maximum of their modulus): values from the fits at several azimuths, FDMNES calculation, and double-Lorentzian model (DL). In the case of $CoCO_3$, the FDMNES calculations are shown for three different convolution parameters, matching three of the experimental curves. The fourth cuvre ($\psi = 50°$) cannot be well fitted with FDMNES calculations. In the case of $NiCO_3$, a single Lorentzian is used to fit the spectra. The yellow vertical dash lines mark the energies shown in Fig. 2 of the letter.

## Results

The main calculated magnetic properties for all considered compounds are listed in Table II. For these calculations, the initial magnetisation directions were set to lie along $x$ direction, which results in having a canted antiferromagnetic state, which is the lowest-energy state for all the systems.

Here we have to emphasize that the values of total magnetic moments shown in Table II are projections of the magnetisation density onto a sphere around the corresponding ion. Due to covalent bonding of $3d$ orbitals of transition metal with $2p$ state of oxygen, part of the magnetisation density appears on the ligand sites. The latter also contributes both to the net magnetic moment and to the estimation of the canting angle. Another important effect of the covalent bonding is the deviation of the calculated $3d$-shell occupation ($N_{3d}$) from the ionic values, which is strongest in the case of $FeBO_3$.

As was shown in the body of the article, the first-principles calculations are able to reproduce the signs of the magnetic chirality in all the systems under consideration. We have done few additional calculations for $MnCO_3$, varying the values of $U$ in a reasonable range, considering the values of 0 (i.e. LSDA+SO), 3, 4 or 5 eV. These calculations confirmed that the sign of DMI is very robust and does not depend on the precise value of $U$, even when it was set to zero. However, the absolute values of the canting angle are significantly influenced by the changes of $U$. As a general trend, we report that larger values of $U$ lead to the suppression of the weak fer-

TABLE II. Calculated total magnetic moment projections (in $\mu_B$) for all considered weak ferromagnets. The contributions of the ligand atoms are summed up. The first $3d$ metal atom is located at the origin, while the second one is at (1/3,2/3,1/6) in the hexagonal setting. The canting angle $\phi$ is calculated as $\arctan(M_y/M_x)$ with the appropriate sign. The corresponding magnetic configurations are visualized in Fig. 1.

| Compound | $N_{3d}$ | atom | $M_x$ | $M_y$ | $M_z$ | Canting angle $\phi$ (deg.) | sgn($\phi$)[7, 38] |
|---|---|---|---|---|---|---|---|
| | | Mn1 | 4.503 | 0.004 | 0 | | |
| $MnCO_3$ | 5.0 | Mn2 | -4.503 | 0.004 | 0 | -0.05 | - |
| | | Ligands | 0 | 0 | 0 | | |
| | | Fe1 | 4.138 | 0.057 | 0 | | |
| $FeBO_3$ | 5.8 | Fe2 | -4.138 | 0.057 | 0 | -0.8 | |
| | | Ligands | 0 | 0.013 | 0 | | |
| | | Co1 | -3.314 | 0.274 | 0.023 | | |
| $CoCO_3$ | 7.1 | Co2 | 3.314 | 0.274 | -0.023 | 4.7 | |
| | | Ligands | 0 | 0.041 | 0 | | |
| | | Ni1 | -1.792 | 0.233 | 0 | | |
| $NiCO_3$ | 8.2 | Ni2 | 1.792 | 0.233 | 0 | 7.4 | + |
| | | Ligands | 0 | 0.054 | 0 | | |

romagnetism. This is probably related to the fact that the larger localisation of the density results into diminishing of the role of the environment on the $3d$ states of the transition metal. As a result, the system is pushed towards an atomic limit, where the anisotropic effects, like DMI and magnetocrystalline anisotropy become less important.

We also report that the use of another realisation of the LSDA+$U$ scheme, suggested in Ref. [39] resulted into an enhanced values of the orbital moments and the canting angles. In case of $MnCO_3$ for the same choice of $U$ and $J$ parameters we obtained twice larger transverse components of the magnetisation as compared with the results of Dudarev's LSDA+$U$ realisation. Present result is naturally explained by the fact that the shape of the $U$-matrix given in Ref. [39] is more complex and allows for more possibilities of the symmetry breaking of the electronic states. Hence, orbital polarisation, which gives rise to anisotropic magnetic interactions, becomes more pronounced in this case.

In Table II we also provide the sign of the DMI predicted theoretically by Moskvin *et al.* [7, 38] for $Fe^{3+}$–$Fe^{3+}$ pair ($d^5-d^5$ electronic configuration) and $Ni^{2+}$-$Ni^{2+}$ pair ($d^8-d^8$) in orthoferrites. These results are obtained from a model approach based on the superexchange theory, which establishes the connection between the DMI sign and the occupation of the $3d$ shell of the transition metals. Numerous parameters that are to be defined in the model scheme hinder a complete quantitative description of the canting state. Nonetheless, our results suggest that the results of Moskvin *et al.* are in qualitative agreement with our first-principles-derived data and therefore is likely to be applicable to other systems, as far as the DMI sign is concerned.

Thus, all the properties of weak ferromagnetism in transition metal carbonates, such as the sign, symmetry and magnitude of DMI can be fully described by means of the all-electron first-principles LSDA+$U$+SO calculations.

## MICROSCOPIC MODEL FOR DMI SIGN CHANGE

To give a microscopic explanation of the dependence of the DMI sign on the occupation of the $3d$ shell we used a toy tight-binding model that contains two atoms having two non-degenerated orbitals of $n(n')$ and $m(m')$ symmetry. The schematic representation of the considered model with the allowed hopping paths is presented in FIG. 8. For simplicity, we assume that the hoppings between the orbitals of the same symmetry are the same, $t_{12}^{mm'} = t_{12}^{nn'}$. The situation with the hoppings between the orbitals of different symmetry is more complicated, since their relation defines the DMI in the system. Importantly, we fix the hopping integrals in our consideration, which means that geometry of the model system does not change.

*DM interaction.* To define the DMI we used the superexchange approach proposed by Moriya [40]:

$$\mathbf{D}_{ij}^{nn'} = \frac{8i}{U}[t_{ij}^{nn'}\mathbf{C}_{ji}^{n'n} - \mathbf{C}_{ij}^{nn'}t_{ji}^{n'n}], \qquad (18)$$

where $t_{ij}^{nn'}$ is the (unperturbed) hopping integral between $n^{th}$ ground orbital state of $i^{th}$ atom and $n'^{th}$ orbital state of $j^{th}$ atom, $\mathbf{C}_{ij}^{nn'}$ is the corresponding hopping renormalised by SOC and $U$ is the on-site Coulomb interaction. Here we assume that one deals with a S=1/2 system.

In case the transition metal oxide the crystal field splitting is much larger that the spin-orbit interaction. It means the latter can be treated as a perturbation. Thus $\mathbf{C}_{ji}^{n'n}$ is given by

$$\mathbf{C}_{ji}^{n'n} = -\frac{\lambda}{2}[\frac{(\mathbf{L}_j^{m'n'})^*}{\epsilon_j^{m'}-\epsilon_j^{n'}}t_{ji}^{m'n} + \frac{\mathbf{L}_i^{mn}}{\epsilon_i^{m}-\epsilon_i^{n}}t_{ji}^{n'm}], \qquad (19)$$

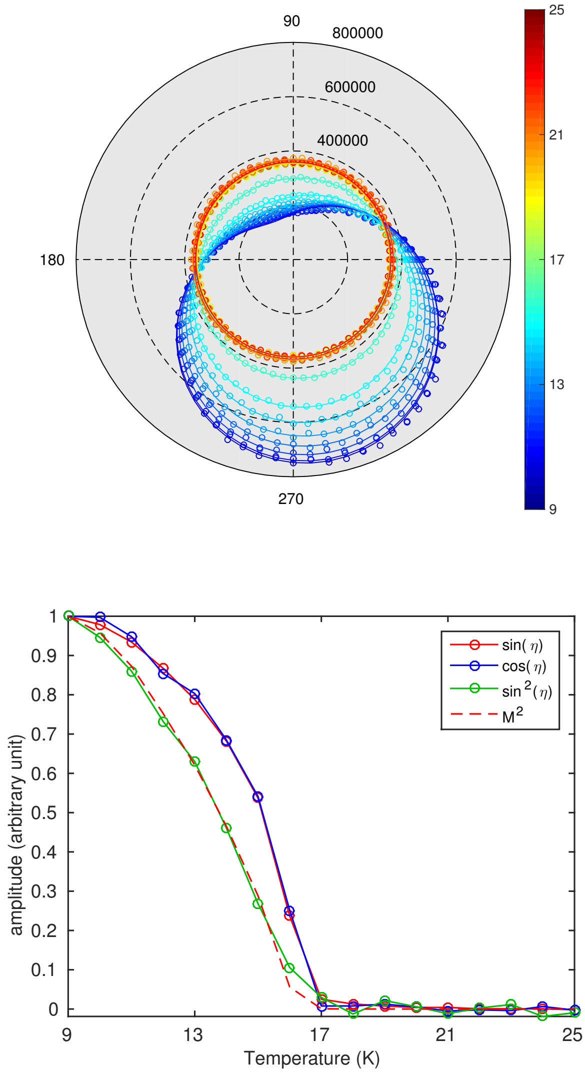


FIG. 7. Top: polar plot (angle: $\eta$, radius: intensity) of the $\eta$-scans recorded at varying temperature on the 009 reflection of $CoCO_3$ ($E = 7.7083$ keV, $\psi = 49.5°$, without polarisation analysis). Experimental data are shown with open circles and the trigonometric fits with plain lines. Bottom: corresponding trigonometric coefficients (normalized to the lowest temperature data point). The curve labelled $M^2$ is the square of the $\sin \eta$ term.

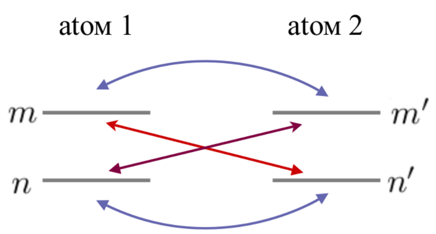


FIG. 8. The proposed toy tight-binding model for explaining the DMI sign change in the carbonates. The horizontal lines represent the electron levels and hopping paths are shown with arrows.

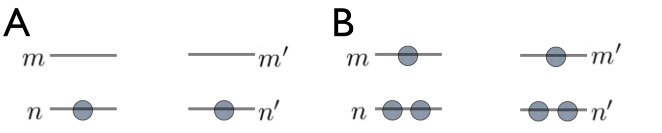


FIG. 9. Two antiferromagnetic ground states corresponding to the S=1/2 systems, obtained in a toy model for different orbital fillings: N=2 (left, A) and N=6 (right, B).

where $\lambda$ is the spin-orbit coupling constant, $\mathbf{L}_i^{mn}$ is the matrix element of the orbital angular momentum between the $m$th excited state and the $n$th ground state Wannier functions which are centered at $i$th ion, while $\epsilon_i^n$ represents the energy of the $n$th Wannier orbital at the $i$th ion.

*S=1/2 system with different occupations.* For our tight-binding model we can define two ground states with different occupations that correspond to S=1/2 case. They are presented in FIG. 9. In the case of N=2 the ground state magnetic orbital is of $n(n')$ symmetry, while for N=6 it is $m(m')$. Another difference between these setups is the different occupations of the excited states. They are empty and fully occupied for N=2 and N=6, respectively.

The difference in the DMIs for N=2 and N=6 occupations is related to the difference between $\mathbf{C}_{21}^{n'\,n}$ and $\mathbf{C}_{21}^{m'\,m}$,

$$\mathbf{C}_{21}^{n'\,n} = -\frac{\lambda}{2}\left[\frac{(\mathbf{L}_2^{m'\,n'})^*}{\epsilon_2^{m'} - \epsilon_2^{n'}} t_{21}^{m'\,n} + \frac{\mathbf{L}_1^{m\,n}}{\epsilon_1^{m} - \epsilon_1^{n}} t_{21}^{n'\,m}\right], \quad (20)$$

$$\mathbf{C}_{21}^{m'\,m} = -\frac{\lambda}{2}\left[\frac{(\mathbf{L}_2^{n'\,m'})^*}{\epsilon_2^{n'} - \epsilon_2^{m'}} t_{21}^{n'\,m} + \frac{\mathbf{L}_1^{n\,m}}{\epsilon_1^{n} - \epsilon_1^{m}} t_{21}^{m'\,n}\right]. \quad (21)$$

Using the relations for the orbital moment elements $\mathbf{L}^{m\,n} = -(\mathbf{L}^{m\,n})^*$, $\mathbf{L}^{m\,n} = -\mathbf{L}^{n\,m}$ and $\Delta E = \epsilon_i^n - \epsilon_i^m$ we rewrite Eqs.(20) - (21) in the following form:

$$\mathbf{C}_{21}^{n'\,n} = -\frac{\lambda \mathbf{L}^{mn}}{2\Delta E}(t_{21}^{m'\,n} - t_{21}^{n'\,m}), \quad (22)$$

$$\mathbf{C}_{21}^{m'\,m} = -\frac{\lambda \mathbf{L}^{mn}}{2\Delta E}(t_{21}^{n'\,m} - t_{21}^{m'\,n}). \quad (23)$$

It means that $\mathbf{C}_{21}^{n'\,n} = -\mathbf{C}_{21}^{m'\,m}$ and $\mathbf{D}_{ij}^{nn'}$ (N=2) = -$\mathbf{D}_{ij}^{mm'}$ (N=6). The absolute values of $\mathbf{D}_{ij}$ (N=2) and $\mathbf{D}_{ij}$ (N=6) will be different if the hoppings $t_{12}^{m\,m'}$ and $t_{12}^{n\,n'}$ are different. Thus, on the level of the Moriya's approach, the sign of the DM interaction depends on the occupation of the excited states. In the case of the carbonates there are both types of the superexchange processes. Depending on the symmetry and occupation, each pair of the $3d$

orbitals can result in positive or negative contribution to the total DMI between two atoms.

---


[1] O. Muller, M. P. O'Horo, and J. F. O'Neill, Journal of Solid State Chemistry **23**, 115 (1978).
[2] I. Maartense, Phys. Rev. **188**, 924 (1969).
[3] I. Maartense, Phys. Rev. B **6**, 4324 (1972).
[4] A. S. Moskvin and M. A. Vigura, Sov. Phys. Solid State **28**, 1268 (1986).
[5] T. Bither, C. G. Frederick, T. Gier, J. Weiher, and H. Young, Solid State Communications **8**, 109 (1970).
[6] R. A. Alikhanov, Soviet Physics JETP **9**, 1204 (1959).
[7] A. S. Moskvin, M. A. Vigura, and A. P. Agafonov, Sov. Phys. Solid State **28**, 1631 (1986).
[8] A. S. Borovik-Romanov, Soviet Physics JETP **9**, 539 (1959).
[9] M. P. Petrov, G. A. Smolensky, A. P. Paugurt, and S. A. Kizhaev, AIP Conference Proceedings **5**, 379 (1972).
[10] U. Köbler, A. Hoser, J. Bos, W. Schäfer, and L. Pohlmann, Physica B: Condensed Matter **355**, 90 (2005).
[11] V. Dmitrienko, E. Ovchinnikova, S. Collins, G. Nisbet, G. Beutier, Y. Kvashnin, V. Mazurenko, A. Lichtenstein, and M. Katsnelson, Nature Physics **10**, 202 (2014).
[12] A. S. Borovik-Romanov and V. I. Ozhogin, Soviet Physics JETP **12**, 18 (1961).
[13] J. Kaczer, Soviet Physics JETP **16**, 1443 (1963).
[14] V. Ozhogin, Soviet Physics JETP **18**, 1156 (1964).
[15] N. M. Kreines and T. A. Shal'Nikova, Soviet Physics JETP **31**, 280 (1970).
[16] A. Bazhan, Soviet Physics JETP **39**, 531 (1974).
[17] Pincini *et al.*, in preparation.
[18] J. Brown, private communication (2014).
[19] Kokubun *et al.*, in preparation.
[20] M. Blume, "Resonant anomalous x-ray scattering," (Elsevier, 1994) Chap. Magnetic Effects in Anomalous Dispersion, p. 495.
[21] S. Grenier and Y. Joly, Journal of Physics: Conference Series **519**, 012001 (2014).
[22] F. de Bergevin and M. Brunel, Acta Crystallographica Section A **37**, 314 (1981).
[23] G. Beutier, E. Ovchinnikova, S. P. Collins, V. E. Dmitrienko, J. E. Lorenzo, J.-L. Hodeau, A. Kirfel, Y. Joly, A. A. Antonenko, V. A. Sarkisyan, and A. Bombardi, Journal of Physics: Condensed Matter **21**, 265402 (2009).
[24] J. P. Hill and D. F. McMorrow, Acta Crystallographica Section A **52**, 236 (1996).
[25] V. E. Dmitrienko, E. N. Ovchinnikova, S. P. Collins, G. Nisbet, and G. Beutier, Journal of Physics: Conference Series **519**, 012003 (2014).
[26] Y. Joly, O. Bunău, J. E. Lorenzo, R. M. Galéra, S. Grenier, and B. Thompson, Journal of Physics: Conference Series **190**, 012007 (2009).
[27] E. Maslen, V. Streltsov, N. Streltsova, and N. Ishizawa, Acta Crystallographica Section B: Structural Science **51**, 929 (1995).
[28] R. Diehl, Solid State Communications **17**, 743 (1975).
[29] F. Pertlik, Acta Crystallographica Section C: Crystal Structure Communications **42**, 4 (1986).
[30] Y. Joly, Phys. Rev. B **63**, 125120 (2001).
[31] D. Treves, Journal of Applied Physics **36**, 1033 (1965), http://dx.doi.org/10.1063/1.1714088.
[32] M. Blume and D. Gibbs, Phys. Rev. B **37**, 1779 (1988).
[33] G. Kresse and J. Furthmüller, Phys. Rev. B **54**, 11169 (1996).
[34] I. V. Solovyev, A. I. Liechtenstein, and K. Terakura, Phys. Rev. Lett. **80**, 5758 (1998).
[35] P. E. Blöchl, Phys. Rev. B **50**, 17953 (1994).
[36] G. Kresse and D. Joubert, Phys. Rev. B **59**, 1758 (1999).
[37] S. L. Dudarev, G. A. Botton, S. Y. Savrasov, C. J. Humphreys, and A. P. Sutton, Phys. Rev. B **57**, 1505 (1998).
[38] A. Moskvin, Journal of Magnetism and Magnetic Materials **400**, 117 (2016), proceedings of the 20th International Conference on Magnetism (Barcelona) 5-10 July 2015.
[39] A. I. Liechtenstein, V. I. Anisimov, and J. Zaanen, Phys. Rev. B **52**, R5467 (1995).
[40] T. Moriya, Phys. Rev. **120**, 91 (1960).
